# Supplementary material for: Scaling up Multi-Turn Off-Policy RL and Multi-Agent Tree Search for LLM Step-Provers
Source: arXiv:2509.06493 source file (2025-10-09)
Supplement: Supplementary file 1 [file appendix.tex]

\section{Hello World}
%\subsection{Hello World}
